# Supplementary material for: Polling Latent Opinions: A Method for Computational Sociolinguistics Using Transformer Language Models
Source: arXiv:2204.07483 source file (2022-04-19)
Supplement: Supplementary file 1 [file appendices.tex]

\appendix

\section{Example Appendix}
\label{sec:appendix}

This is an appendix.
